# Supplementary material for: Sequential Relational Decomposition
Source: arXiv:1903.01368 source file (2022-03-02)
Supplement: Supplementary file 1 [file Appendix.tex]

 \input{RegularFDP}
